# Supplementary material for: Understanding Collaborative Practices and Tools of Professional UX Practitioners in Software Organizations
Source: arXiv:2302.11845 source file (2023-02-26)
Supplement: Supplementary file 1 [file appendix.tex]

%TC:ignore
\section{Survey Instrument}
\subsection{Pre-Survey}

Hello! We are researchers from [redacted] interested in understanding how UX practitioners collaborate. We invite you to fill out the following survey. Completion time is expected to be around 10–15 minutes and you will be entered into a raffle to win 1 of 5 \$50 Amazon gift cards upon submitting your responses. We will use your input to research and create new tools for UX collaboration. 

Your participation is voluntary. You may leave any question unanswered, and you may leave the survey at any time. 

This survey is anonymous, unless you choose to provide your email address on the last page of the survey. We will treat all of your responses as confidential. When reporting results, we will use anonymous, aggregated analyses. If you have any questions, please reach out to researcher [redacted] at [redacted]. 

We greatly appreciate your time and look forward to your responses!

Before you proceed to the survey, please complete the captcha below.

[captcha]

\subsection{Intro}

\begin{enumerate}
    
    \item How long have you worked...
        \begin{itemize}
            \item ...as a professional?
                \begin{itemize}
                    \item[o] 0-2 years
                    \item[o] 3-5 years
                    \item[o] 6-10 years
                    \item[o] 11-20 years
                    \item[o] 20+ years
                    \item[o] Prefer not to answer
                \end{itemize}
            \item ...in UX?
                \begin{itemize}
                    \item[o] 0-2 years
                    \item[o] 3-5 years
                    \item[o] 6-10 years
                    \item[o] 11-20 years
                    \item[o] 20+ years
                    \item[o] Prefer not to answer
                \end{itemize}
            \item ...at your current company?
                \begin{itemize}
                    \item[o] 0-2 years
                    \item[o] 3-5 years
                    \item[o] 6-10 years
                    \item[o] 11-20 years
                    \item[o] 20+ years
                    \item[o] Prefer not to answer
                \end{itemize}
        \end{itemize}

    \item What is your job title? [Free-form text]

    \item What is the approximate size of your current employer, in number of employees?
        \begin{itemize}
            \item[o] 0-100
            \item[o] 101-1000
            \item[o] 1001-10,000
            \item[o] 10,001+
        \end{itemize}

    \item How do you describe your gender identity?
        \begin{itemize}
            \item[o] Female
            \item[o] Male
            \item[o] Non-binary / third gender
            \item[o] Prefer not to say
        \end{itemize}
\end{enumerate}

\subsection{Your UX Team}
For the remaining questions in this survey, please think about a recent project
you were involved in and completed.

\begin{enumerate}
    \item Which stage(s) of the design process were you involved in?
        \begin{itemize}
            \item[$\square$] Research (e.g. field work, interviews, user testing)
            \item[$\square$] Synthesis (e.g. analyzing research, defining personas, forming design problem)
            \item[$\square$] Low fidelity design (e.g. sketches, wireframes, storyboards)
            \item[$\square$] High fidelity design (e.g. interactive prototyping, visual refinement, motion/animation)
            \item[$\square$] Communication (e.g. pitches, demos, hand-off)
        \end{itemize}
    \item What was the size of the UX team you worked with on the project (including
yourself)?
        \begin{itemize}
            \item[o] 1 ( just me)
            \item[o] 2-4
            \item[o] 5-7
            \item[o] 8-10
            \item[o] 11+
        \end{itemize}
    \item My UX team was...
    \begin{itemize}
        \item[$\square$] ...standalone and consulted for non-UX teams
        \item[$\square$] ...situated within a larger team that does not exclusively do UX
        \item[$\square$] ...situated within a larger UX team
        \item[$\square$] Other [Free-form text]
    \end{itemize}
    \item In the project, if you/your team designed experiences involving one or more of the following technologies, please indicate them below. If not, or you are not sure, leave this question blank.
    \begin{itemize}
        \item[$\square$] Natural language technologies (e.g. personal assistants, speech-to-text)
        \item[$\square$] Computer vision (e.g. object recognition, photo tagging)
        \item[$\square$] Spam and malware filtering
        \item[$\square$] Recommendation systems
        \item[$\square$] Other AI/machine learning technologies not mentioned above
    \end{itemize}
\end{enumerate}

\subsection{Roles and Collaboration}
Here are some common UX roles:
\begin{itemize}
    \item Designer
    \item Researcher
    \item Engineer
    \item Writer
\end{itemize}

And here are some common non-UX roles:
\begin{itemize}
    \item Product/program manager
    \item Software developer/engineer
    \item Data scientist
    \item Domain expert (people with domain-specific knowledge, e.g. doctor)
    \item Sales/Marketing/Finance
\end{itemize}

\begin{enumerate}
    \item In the project you have in mind, which UX role did you take on? If you took on multiple, select the one you most closely associate with.
        \begin{itemize}
            \item[o] Designer 
            \item[o] Researcher
            \item[o] Engineer
            \item[o] Writer
            \item[o] Other [Free-form text]
        \end{itemize}
    \item At each stage of the design process you were involved in (each row), which roles did you collaborate with? Definitions for the roles can be found at the top of the page.
        \begin{itemize}
            \item Research (e.g. field work, interviews, user testing)
                \begin{itemize}
                    \item[$\square$] UX Designer
                    \item[$\square$] UX Researcher
                    \item[$\square$] UX Engineer
                    \item[$\square$] UX Writer
                    \item[$\square$] Product Manager
                    \item[$\square$] Software Developer
                    \item[$\square$] Data Scientist
                    \item[$\square$] Domain Expert
                    \item[$\square$] Sales / Marketing / Finance
                \end{itemize}
            \item Synthesis (e.g. analyzing research, defining personas, forming design problem)
                \begin{itemize}
                    \item[$\square$] UX Designer
                    \item[$\square$] UX Researcher
                    \item[$\square$] UX Engineer
                    \item[$\square$] UX Writer
                    \item[$\square$] Product Manager
                    \item[$\square$] Software Developer
                    \item[$\square$] Data Scientist
                    \item[$\square$] Domain Expert
                    \item[$\square$] Sales / Marketing / Finance
                \end{itemize}
            \item Low fidelity design (e.g. sketches, wireframes, storyboards)
                \begin{itemize}
                    \item[$\square$] UX Designer
                    \item[$\square$] UX Researcher
                    \item[$\square$] UX Engineer
                    \item[$\square$] UX Writer
                    \item[$\square$] Product Manager
                    \item[$\square$] Software Developer
                    \item[$\square$] Data Scientist
                    \item[$\square$] Domain Expert
                    \item[$\square$] Sales / Marketing / Finance
                \end{itemize}
            \item High fidelity design (e.g. interactive prototyping, visual refinement, motion/animation)
                \begin{itemize}
                    \item[$\square$] UX Designer
                    \item[$\square$] UX Researcher
                    \item[$\square$] UX Engineer
                    \item[$\square$] UX Writer
                    \item[$\square$] Product Manager
                    \item[$\square$] Software Developer
                    \item[$\square$] Data Scientist
                    \item[$\square$] Domain Expert
                    \item[$\square$] Sales / Marketing / Finance
                \end{itemize}
            \item Communication (e.g. pitches, demos, hand-off)
                \begin{itemize}
                    \item[$\square$] UX Designer
                    \item[$\square$] UX Researcher
                    \item[$\square$] UX Engineer
                    \item[$\square$] UX Writer
                    \item[$\square$] Product Manager
                    \item[$\square$] Software Developer
                    \item[$\square$] Data Scientist
                    \item[$\square$] Domain Expert
                    \item[$\square$] Sales / Marketing / Finance
                \end{itemize}
        \end{itemize}

    \item Briefly, what are some strategies you used to document and explain your design decisions to \textbf{other UXers?} [Free-form text]

    \item Briefly, what are some strategies you used to document and explain your design decisions to \textbf{non-UXers?} [Free-form text]

    \item How did \textbf{collaborations with non-UXers} typically begin?
    \begin{itemize}
        \item[o] Non UXers initiated collaboration because they wanted UX input
        \item[o] I/my team initiated collaboration because I/we wanted others' input
        \item[o] N/A: I didn't collaborate with non-UXers
        \item[o] Other [Free-form text]
    \end{itemize}
\end{enumerate}

\subsection{Branch: Non-Design}
\textit{This branch was accessed instead of the Design branch if participants did not engage in low- or high-fidelity design.}
    \subsubsection{Design and Collaboration Tools}
    \begin{enumerate}
        \item What tool(s) did you use to \textbf{synthesize research and generate ideas}? If you used multiple, please list the most-used ones first. [Free-form text]
        
        \item Did you collaborate with others in the above tool(s)? If yes, please briefly describe how you did so.
        
        \item What tool(s) did you use to \textbf{share and communicate your work}? If you used multiple, please list the most-used ones first. [Free-form text]
        
        \item Did you collaborate with others in the above tool(s)? If yes, please briefly describe how you did so. [Free-form text]
    \end{enumerate}
    
    \subsubsection{AI/ML}
    \textit{This section was only shown if at least one of the options in Q4 of \textbf{Your UX Team} was selected.}
    \begin{enumerate}
        \item What was your understanding of the capabilities and limitations of the ML model(s) behind the project?
            \begin{itemize}
                \item[o] I was very aware of them because I understood the metrics used for model evaluation (e.g. F1 score, ROC AUC)
                \item[o] I was very aware of them because I thoroughly interacted with the model myself
                \item[o] I was very aware of them because others told me about them in detail
                \item[o] I was not very aware of them but had some idea from others telling me about them
                \item[o] I was not very aware of them but had some idea from interacting with the model myself
                \item[o] I was not aware at all
            \end{itemize}
    
        \item If you were not fully aware, what strategies did you use to help you design using the model(s)? [Free-form text]
        
        \item Did you encounter any obstacles to collaborating with relevant stakeholders (e.g. data scientists, engineers, product managers) in this ML project? If so, what were they? [Free-form text]
        
        \item What tools and/or collaborative practices did you wish you had to help you design with ML, if any? [Free-form text]
    \end{enumerate}
    
    \subsubsection{Conclusion: Your Turn}
    \begin{enumerate}
        \item Is there anything else that you would like to tell us about your experiences with collaboration in UX? [Free-form text]

        \item Please provide your email here so we can contact you if you win this survey's raffle: We will not use your email for anything other than logistics for this survey, such as prize distribution. [Free-form text]
        
        \item If you are interested in participating in an interview related to topics in this survey, please indicate the topic(s) you would be interested in talking about. Please also provide your preferred contact method below if it is different from the email you entered previously. You will receive a separate prize gift upon completion of the interview, in addition to being entered into this survey's raffle.
        \begin{itemize}
            \item[$\square$] Design and Collaboration Tools
            \item[$\square$] Developer Hand-Off
            \item[$\square$] Design Systems and Reusing Designs
            \item[$\square$] AI/ML
            \item[$\square$] Please provide your preferred contact here (if different from email) [Free-form text]
        \end{itemize}
        
        \item Finally, if you are interested in seeing a report from this research project once it's completed, please provide your email here: [Free-form text]
    \end{enumerate}
    
\subsection{Branch: Design}
\textit{This branch was accessed instead of the Non-Design branch if participants engaged in low- or high-fidelity design.}
    \subsubsection{Design and Collaboration Tools}
    \begin{enumerate}
        \item What tool(s) did you use to \textbf{synthesize research and generate ideas}? If you used multiple, please list the most-used ones first. [Free-form text]
        
        \item Did you collaborate with others in the above tool(s)? If yes, please briefly describe how you did so.
        
        \item What tool(s) did you use to \textbf{create low-fidelity designs}? If you used multiple, please list the most-used ones first. [Free-form text]
        
        \item Did you collaborate with others in the above tool(s)? If yes, please briefly describe how you did so. [Free-form text]
        
        \item What tool(s) did you use to \textbf{create high-fidelity designs}? If you used multiple, please list the most-used ones first. [Free-form text]
        
        \item Did you collaborate with others in the above tool(s)? If yes, please briefly describe how you did so. [Free-form text]
        
        \item What tool(s) did you use to \textbf{share and communicate your work}? If you used multiple, please list the most-used ones first. [Free-form text]
        
        \item Did you collaborate with others in the above tool(s)? If yes, please briefly describe how you did so. [Free-form text]
    \end{enumerate}

    \subsubsection{AI/ML}
    \textit{This section was only shown if at least one of the options in Q4 of \textbf{Your UX Team} was selected.}
    \begin{enumerate}
        \item What was your understanding of the capabilities and limitations of the ML model(s) behind the project?
            \begin{itemize}
                \item[o] I was very aware of them because I understood the metrics used for model evaluation (e.g. F1 score, ROC AUC)
                \item[o] I was very aware of them because I thoroughly interacted with the model myself
                \item[o] I was very aware of them because others told me about them in detail
                \item[o] I was not very aware of them but had some idea from others telling me about them
                \item[o] I was not very aware of them but had some idea from interacting with the model myself
                \item[o] I was not aware at all
            \end{itemize}
    
        \item If you were not fully aware, what strategies did you use to help you design using the model(s)? [Free-form text]
        
        \item Did you encounter any obstacles to collaborating with relevant stakeholders (e.g. data scientists, engineers, product managers) in this ML project? If so, what were they? [Free-form text]
        
        \item What tools and/or collaborative practices did you wish you had to help you design with ML, if any? [Free-form text]
    \end{enumerate}
    
    \subsubsection{Design Environment Customization}
    \begin{enumerate}
        \item Did you install tool plugins to customize your design environment?
        \begin{itemize}
            \item[o] Yes, I used plugins built by those in my company (including myself)
            \item[o] Yes, I used plugins built by others outside of my company
            \item[o] Yes, I used plugins from both in and outside of my company
            \item[o] Yes, I used plugins, but am not sure who built them
            \item[o] No
        \end{itemize}

        \item How did you first you hear about the plugins you installed?
        \begin{itemize}
            \item[o] I wanted a certain functionality so I searched for the plugin myself
            \item[o] I heard about it from someone in my company
            \item[o] I heard about it from someone outside of my company
        \end{itemize}
        
        \item How often did you encounter situations in which you can perform certain actions in your design environment because of your plugin(s), but your collaborators (who work in the same file as you) can't?
        \begin{itemize}
            \item[o] Very often
            \item[o] Sometimes
            \item[o] Rarely or never
        \end{itemize}
        
        \item How did you deal with the situation mentioned in the previous question when it occurred? The situation was: you can perform certain actions in your design environment because of your plugin(s), but your collaborators (who work in the same file as you) can't.
        \begin{itemize}
            \item[o] I tell them to install the plugin(s) I have
            \item[o] I do all the actions that need to be done using the plugins on their behalf
            \item[o] I ignore it since it's not much of a problem
            \item[o] Other [Free-form text]
        \end{itemize}
    \end{enumerate}
    
    \subsubsection{Pre-handoff: Developer Hand-Off}
    \begin{enumerate}
        \item Did you share your designs with developers for them to implement?
        \begin{itemize}
            \item[o] Yes
            \item[o] No
        \end{itemize}
    \end{enumerate}
    
    \subsubsection{Hand-off: Developer Hand-Off}
    \textit{This section was only shown if answer to previous question was ``Yes.''}
    \begin{enumerate}
        \item What artifacts did you pass along to developers for them to implement your design(s)?
        \begin{itemize}
            \item[$\square$] Written design spec
            \item[$\square$] High fidelity prototype
            \item[$\square$] Low fidelity prototype
            \item[$\square$] My entire design file
            \item[$\square$] Code snippets (HTML/CSS/JavaScript)
            \item[$\square$] Other [Free-form text]
        \end{itemize}
        
        \item Was there anything you did to your designs to make sure developers can understand and implement them? If so, briefly outline what you did [Free-form text]
        
        \item Do you think it's important for developers to implement interfaces that aligned with your designs?
        \begin{itemize}
            \item[o] It's very important—my designs should be pretty close to the look and feel of the implementation
            \item[o] It's kind of important—my designs should be treated as recommended guidelines
            \item[o] It's not really important—developers can follow my designs when they see fit
            \item[o] It's not important at all—I don't care if developers use my designs
        \end{itemize}
        
        \item What was your role after you handed off your design(s) to developers?
        \begin{itemize}
            \item[o] I work closely with developers to help them implement it
            \item[o] I occasionally answer questions from developers and make changes if requested
            \item[o] I don't do anything more
            \item [o] Other [Free-form text]
        \end{itemize}
        
        \item How different was the actual implementation from your designs?
        \begin{itemize}
            \item[o] It's very similar or even identical to the way I designed it
            \item[o] It's a bit different—some design changes needed to be made
            \item[o] It's very different—major design changes needed to be made
            \item[o] I don't know—I didn't see the implementation
        \end{itemize}
        
        \item In scenarios where the design and implementation diverged, what did you do?
        \begin{itemize}
            \item[o] I "caught up" with the implementation by re-doing some of my designs
            \item[o] I "caught up" with the implementation by designing off of screenshots and discarding my old designs
            \item[o] I continued using my old designs, keeping in mind that they are different from the implementation
            \item[o] I ignored the difference
            \item[o] I was not involved after they diverged
            \item[o] Other [Free-form text]
        \end{itemize}
        
        \item In general (beyond the project you have in your mind), how often did design and implementation diverge?
        \begin{itemize}
            \item[o] Almost all the time
            \item[o] Some of the time
            \item[o] Rarely or never
            \item[o] I don't know—I'm usually no longer involved after hand-off
        \end{itemize}
    \end{enumerate}
    
    \subsubsection{Design Reuse and Design Systems}
    \begin{enumerate}
        \item If you worked with a design system in your project, what was your relationship with it? If you did not work with a design system, please leave this blank.
        \begin{itemize}
            \item[$\square$] I used assets from the design system
            \item[$\square$] I contributed assets to the design system
            \item[$\square$] Other [Free-form text]
        \end{itemize}
        
        \item Did you use designs created by others as part of your project?
        \begin{itemize}
            \item[o] Yes, I used designs from other UXers in my company
            \item[o] Yes, I used designs from others outside of my company
            \item[o] Yes, I used designs from both inside and outside of my company
            \item[o] No
        \end{itemize}
        
        \item Did you expect other UXers to reuse or build off of your designs?
        \begin{itemize}
            \item[o] Yes
            \item[o] No
        \end{itemize}
        
        \item What are some challenges you observed in getting design systems adopted widely by your collaborators, if any? [Free-form text]
    \end{enumerate}
    
    \subsubsection{Conclusion: Your Turn}
    \begin{enumerate}
        \item Is there anything else that you would like to tell us about your experiences with collaboration in UX? [Free-form text]
        
        \item Please provide your email here so we can contact you if you win this survey's raffle: We will not use your email for anything other than logistics for this survey, such as prize distribution. [Free-form text]
        
        \item If you are interested in participating in an interview related to topics in this survey, please indicate the topic(s) you would be interested in talking about. Please also provide your preferred contact method below if it is different from the email you entered previously. You will receive a separate prize gift upon completion of the interview, in addition to being entered into this survey's raffle.
        \begin{itemize}
            \item[$\square$] Design and Collaboration Tools
            \item[$\square$] Developer Hand-Off
            \item[$\square$] Design Systems and Reusing Designs
            \item[$\square$] AI/ML
            \item[$\square$] Please provide your preferred contact here (if different from email) [Free-form text]
        \end{itemize}
        
        \item If you would like to be emailed a copy of the research report from this study once it is available, please check the box below
        \begin{itemize}
            \item[$\square$] Yes, I'd like a copy of the report when available
        \end{itemize}
    \end{enumerate}

    %TC:endignore
